# Supplementary material for: Pre-trained Model Guided Fine-Tuning for Zero-Shot Adversarial Robustness
Source: arXiv:2401.04350 source file (2024-04-10)
Supplement: Supplementary file 1 [file X_suppl.tex]

\clearpage
\setcounter{page}{1}
\maketitlesupplementary

% % 
% Having the supplementary compiled together with the main paper means that:
% % 
% \begin{itemize}
% \item The supplementary can back-reference sections of the main paper, for example, we can refer to \cref{sec:intro};
% \item The main paper can forward reference sub-sections within the supplementary explicitly (e.g. referring to a particular experiment); 
% \item When submitted to arXiv, the supplementary will already included at the end of the paper.
% \end{itemize}
% % 
% To split the supplementary pages from the main paper, you can use \href{https://support.apple.com/en-ca/guide/preview/prvw11793/mac#:~:text=Delete%20a%20page%20from%20a,or%20choose%20Edit%20%3E%20Delete).}{Preview (on macOS)}, \href{https://www.adobe.com/acrobat/how-to/delete-pages-from-pdf.html#:~:text=Choose%20%E2%80%9CTools%E2%80%9D%20%3E%20%E2%80%9COrganize,or%20pages%20from%20the%20file.}{Adobe Acrobat} (on all OSs), as well as \href{https://superuser.com/questions/517986/is-it-possible-to-delete-some-pages-of-a-pdf-document}{command line tools}.

\begin{table*}[htbp]
\centering
\caption{Adversarial zero-shot robust accuracies under PGD-10 \cite{madry2017towards} attack. We fine-tune the model on CIFAR100 \cite{krizhevsky2009learning} and evaluate six methods (rows) on 16 datasets (columns), presenting the accuracy for each dataset as well as the average accuracy, with the best results shown in bold. 
Here, CLIP represents the pre-trained CLIP model, while FT-standard refers to the model fine-tuned on clean datasets.}
\label{tab:cifar-robust}
\begin{adjustbox}{width=\textwidth,keepaspectratio}
\begin{tabular}{lcccccccccccccccccc}
\toprule
% & \multicolumn{16}{c}{\textbf{Datasets}} \\ % 合并中间的列，并在合并的列上添加标题 "Datasets"
% \cmidrule(lr){2-17} % 这个命令将会在从第二列到第十三列的上方画一条线，'lr'是为了减少线的长度
Method    & \scriptsize\rotatebox{90}{CIFAR10 (\%)} & \scriptsize\rotatebox{90}{CIFAR100 (\%)} & \scriptsize\rotatebox{90}{STL10 (\%)} & \scriptsize\rotatebox{90}{SUN397 (\%)} & \scriptsize\rotatebox{90}{Food101 (\%)} & \scriptsize\rotatebox{90}{Oxfordpet (\%)} & \scriptsize\rotatebox{90}{Flowers102 (\%)} & \scriptsize\rotatebox{90}{DTD (\%)}   & \scriptsize\rotatebox{90}{EuroSAT (\%)} & \scriptsize\rotatebox{90}{Fgvc\_Aircraft (\%)} & \scriptsize\rotatebox{90}{TinyImageNet (\%)} & \scriptsize\rotatebox{90}{ImageNet (\%)} & \scriptsize\rotatebox{90}{Caltech101 (\%)} & \scriptsize\rotatebox{90}{Caltech256 (\%)} & \scriptsize\rotatebox{90}{StanfordCars (\%)} & \scriptsize\rotatebox{90}{PCAM (\%)}  & Average (\%) & Time (s) \\ 
\midrule
CLIP           & 45.70          & 19.53          & 68.35          & 9.62           & 3.12          & 9.76           & 3.51           & 21.87          & 3.64           & 0.39           & 0.39          & 6.44           & 15.62          & 23.11          & 2.73          & 50.27          & 17.75    &0 \\ \hline
FT-Standard    & 27.34          & 15.43          & 57.03          & 10.01          & 3.20          & 5.85           & 4.10           & 17.18          & 0.65           & 0.00           & 0.00          & 6.83           & 16.60          & 22.46          & 2.53          & 35.65          & 14.05  &101 \\
FT-TeCoA \cite{mao2022understanding}       & 58.20          & \textbf{39.25} & 66.40          & 13.79          & 4.60          & 11.71          & 9.76           & 21.09          & 11.13          & 0.39           & 1.17          & 8.90           & 18.94          & 29.10          & 5.26          & 41.96          & 21.35  &253 \\
PMG-AFT (ours)         & \textbf{64.06} & 36.33          & \textbf{70.12} & \textbf{17.93} & \textbf{7.50} & \textbf{22.66} & \textbf{10.55} & \textbf{30.86} & \textbf{22.92} & \textbf{1.17}  & \textbf{2.73} & \textbf{10.51} & \textbf{21.09} & \textbf{34.83} & \textbf{5.46} & \textbf{58.37} & \textbf{26.06}  & 377\\ \hline
VP-TeCoA  \cite{mao2022understanding}     & 54.68          & 37.89          & 47.26          & 6.15           & 1.95          & 5.46           & 10.15          & 1.56           & 0.21           & 0.00           & 2.14          & 3.82           & 13.27          & 15.43          & 0.97          & 52.12          & 15.81  & 350\\
VPT-PMG-AFT (ours)         & \textbf{61.52} & \textbf{41.01} & \textbf{53.90}  & \textbf{8.24}  & \textbf{3.51} & \textbf{7.81}  & \textbf{10.41} & \textbf{2.34}  & \textbf{0.85}  & \textbf{1.17}  & \textbf{2.53} & \textbf{5.35}  & \textbf{13.47}          & \textbf{28.90 }         & \textbf{3.32}         & \textbf{55.16}          & \textbf{18.71}  &670\\
\bottomrule
\end{tabular}
\end{adjustbox}
\vspace{-3mm}
\end{table*}
\begin{table*}[htbp]
\centering
\caption{Zero-shot clean accuracies. 
We fine-tune the model on CIFAR100 \cite{krizhevsky2009learning} and evaluate six methods (rows) on 16 datasets (columns), presenting the accuracy for each dataset as well as the average accuracy.
After fine-tuning or adversarial fine-tuning on CIFAR100 \cite{krizhevsky2009learning}, the zero-shot accuracy of the CLIP model on clean images generally decreases.}
\label{tab:cifar-clean}
\begin{adjustbox}{width=\textwidth,keepaspectratio}
\begin{tabular}{lcccccccccccccccccc}
\toprule
% & \multicolumn{16}{c}{\textbf{Datasets}} \\ % 合并中间的列，并在合并的列上添加标题 "Datasets"
% \cmidrule(lr){2-17} % 这个命令将会在从第二列到第十三列的上方画一条线，'lr'是为了减少线的长度
Method    & \scriptsize\rotatebox{90}{CIFAR10 (\%)} & \scriptsize\rotatebox{90}{CIFAR100 (\%)} & \scriptsize\rotatebox{90}{STL10 (\%)} & \scriptsize\rotatebox{90}{SUN397 (\%)} & \scriptsize\rotatebox{90}{Food101 (\%)} & \scriptsize\rotatebox{90}{Oxfordpet (\%)} & \scriptsize\rotatebox{90}{Flowers102 (\%)} & \scriptsize\rotatebox{90}{DTD (\%)}   & \scriptsize\rotatebox{90}{EuroSAT (\%)} & \scriptsize\rotatebox{90}{Fgvc\_Aircraft (\%)} & \scriptsize\rotatebox{90}{TinyImageNet (\%)} & \scriptsize\rotatebox{90}{ImageNet (\%)} & \scriptsize\rotatebox{90}{Caltech101 (\%)} & \scriptsize\rotatebox{90}{Caltech256 (\%)} & \scriptsize\rotatebox{90}{StanfordCars (\%)} & \scriptsize\rotatebox{90}{PCAM (\%)}  & Average (\%) & Time (s) \\ 
\midrule
CLIP          & 88.28          & 63.47          & 97.65          & 55.06          & 76.79          & 85.93         & 48.43          & 43.75          & 45.31          & 8.20           & 59.18          & 62.65          & 32.22          & 86.13          & 54.10          & 52.67          & 59.98 & 0 \\ \hline
FT-Standard   & 91.21          & 77.73          & 97.46          & 55.02          & 68.82          & 84.37         & 38.86          & 43.75          & 37.82          & 13.28          & 49.21          & 54.49          & 28.71          & 78.12          & 49.41          & 46.15          & 57.15 &101 \\
FT-TeCoA \cite{mao2022understanding}      & 85.93   & 69.53    & 95.31 & 55.04  & 69.60   & 85.54     & 37.89      & 42.57 & 32.16   & 8.59           & 50.78        & 56.60         & 28.12        & 80.99 & 51.56 & 45.14 & 55.95 &253 \\
PMG-AFT (ours)         & 80.86   & 60.15    & 95.31 & 57.12  & 72.81   & 83.20     & 41.40      & 42.58 & 31.32   & 8.20           & 46.48        & 60.15         & 30.85        & 84.04 & 54.49 & 58.03 & 56.68 &377 \\ \hline
VPT-TeCoA \cite{mao2022understanding}     & 78.71   & 57.03    & 83.91 & 30.92  & 24.76   & 37.89     & 11.97      & 21.09 & 12.57   & 1.56           & 38.08        & 25.00         & 26.36        & 48.11 & 11.52 & 56.30 & 35.36 &350\\
VPT-PMG-AFT (ours)       & 83.59   & 61.13    & 85.54 & 38.55  & 39.53   & 49.60     & 16.66      & 33.59 & 13.13   & 14.06          & 40.23        & 33.51         & 24.60        & 61.65 & 23.63 & 59.73 & 42.42 &670\\
\bottomrule
\end{tabular}
\end{adjustbox}
\vspace{-5mm}
\end{table*}
\begin{table*}[htbp]
\centering
\caption{Adversarial zero-shot robust accuracies under PGD-10 \cite{madry2017towards} attack with different perturbation bounds ($\varepsilon=1/255, 2/255$ and $4/255$). We fine-tune the model on TinyImageNet \cite{deng2009imagenet} and evaluate on 16 datasets (columns), presenting the accuracy for each dataset as well as the average accuracy, with the best results shown in bold. We employ the same perturbation bound for both training and testing.}
\label{tab:strength-robust}
\begin{adjustbox}{width=\textwidth,keepaspectratio}
\begin{tabular}{lccccccccccccccccc}
\toprule
% & \multicolumn{16}{c}{\textbf{Datasets}} \\ % 合并中间的列，并在合并的列上添加标题 "Datasets"
% \cmidrule(lr){2-17} % 这个命令将会在从第二列到第十三列的上方画一条线，'lr'是为了减少线的长度
Method    & \scriptsize\rotatebox{90}{CIFAR10 (\%)} & \scriptsize\rotatebox{90}{CIFAR100 (\%)} & \scriptsize\rotatebox{90}{STL10 (\%)} & \scriptsize\rotatebox{90}{SUN397 (\%)} & \scriptsize\rotatebox{90}{Food101 (\%)} & \scriptsize\rotatebox{90}{Oxfordpet (\%)} & \scriptsize\rotatebox{90}{Flowers102 (\%)} & \scriptsize\rotatebox{90}{DTD (\%)}   & \scriptsize\rotatebox{90}{EuroSAT (\%)} & \scriptsize\rotatebox{90}{Fgvc\_Aircraft (\%)} & \scriptsize\rotatebox{90}{TinyImageNet (\%)} & \scriptsize\rotatebox{90}{ImageNet (\%)} & \scriptsize\rotatebox{90}{Caltech101 (\%)} & \scriptsize\rotatebox{90}{Caltech256 (\%)} & \scriptsize\rotatebox{90}{StanfordCars (\%)} & \scriptsize\rotatebox{90}{PCAM (\%)}  & Average (\%) \\ 
\midrule
FT-TeCoA-1/255 \cite{mao2022understanding}          & 40.82 & 24.41 & 70.70 & 19.21 & 14.45& 28.13& 23.05& 28.13 & 12.57& 3.13 & \textbf{19.33}& 16.48& 24.02 & 40.56 & 12.69& 53.68 &26.96     \\
PMG-AFT-1/255(ours)    & \textbf{66.99} & \textbf{38.28} & \textbf{76.17} & \textbf{24.23} & \textbf{14.92}& \textbf{33.59}& \textbf{23.43}& \textbf{34.38} & \textbf{24.15}& \textbf{3.91} & 14.84& \textbf{17.26}& \textbf{24.02} & \textbf{45.05} & \textbf{14.64}& \textbf{57.64} &\textbf{31.95}  \\ \hline
FT-TeCoA-2/255 \cite{mao2022understanding}       & 32.21          & 11.71          & 52.73          & 10.63          & 2.73          & 7.42           & \textbf{14.06} & 24.21          & 16.08          & \textbf{0.39} & \textbf{5.85} & 7.85           & 17.57          & 21.68          & 1.56          & 53.55          & 17.51  \\
PMG-AFT-2/255(ours)         & \textbf{63.28} & \textbf{26.56} & \textbf{66.79} & \textbf{13.83} & \textbf{3.18} & \textbf{7.64}  & 7.81           & \textbf{30.07} & \textbf{21.15} & 0.00             & 4.49          & \textbf{8.07}  & \textbf{18.16} & \textbf{27.66} & \textbf{1.95} & \textbf{54.79} & \textbf{22.21}   \\ \hline
FT-TeCoA-4/255  \cite{mao2022understanding}     & 29.29          & 9.18           & 46.28          & 4.63           & 0.39          & 0.00              & \textbf{0.78}  & 21.48          & 12.95          & 0.00             & 1.75          & 1.36           & 13.67          & 11.78          & 0.00             & 53.51          & 12.94   \\
PMG-AFT-4/255(ours)         & \textbf{63.28} & \textbf{21.87} & \textbf{59.96} & \textbf{7.17}  & \textbf{0.42} & \textbf{0.39}  & 0.58           & \textbf{26.56} & \textbf{20.11} & 0.00             & \textbf{1.95} & \textbf{1.36}  & \textbf{15.03} & \textbf{12.63} & \textbf{0.00}    & \textbf{53.57} & \textbf{17.80}   \\
\bottomrule
\end{tabular}
\end{adjustbox}
\end{table*}
\begin{table*}[htbp]
\centering
\caption{Zero-shot clean accuracies. We fine-tune the model on TinyImageNet \cite{deng2009imagenet} with PGD-10 \cite{madry2017towards} of different perturbation bounds ($\varepsilon=1/255, 2/255$ and $4/255$) and evaluate on 16 datasets (columns), presenting the accuracy for each dataset as well as the average accuracy, with the best average result shown in bold.}
\label{tab:strength-clean}
\begin{adjustbox}{width=\textwidth,keepaspectratio}
\begin{tabular}{lccccccccccccccccc}
\toprule
% & \multicolumn{16}{c}{\textbf{Datasets}} \\ % 合并中间的列，并在合并的列上添加标题 "Datasets"
% \cmidrule(lr){2-17} % 这个命令将会在从第二列到第十三列的上方画一条线，'lr'是为了减少线的长度
Method    & \scriptsize\rotatebox{90}{CIFAR10 (\%)} & \scriptsize\rotatebox{90}{CIFAR100 (\%)} & \scriptsize\rotatebox{90}{STL10 (\%)} & \scriptsize\rotatebox{90}{SUN397 (\%)} & \scriptsize\rotatebox{90}{Food101 (\%)} & \scriptsize\rotatebox{90}{Oxfordpet (\%)} & \scriptsize\rotatebox{90}{Flowers102 (\%)} & \scriptsize\rotatebox{90}{DTD (\%)}   & \scriptsize\rotatebox{90}{EuroSAT (\%)} & \scriptsize\rotatebox{90}{Fgvc\_Aircraft (\%)} & \scriptsize\rotatebox{90}{TinyImageNet (\%)} & \scriptsize\rotatebox{90}{ImageNet (\%)} & \scriptsize\rotatebox{90}{Caltech101 (\%)} & \scriptsize\rotatebox{90}{Caltech256 (\%)} & \scriptsize\rotatebox{90}{StanfordCars (\%)} & \scriptsize\rotatebox{90}{PCAM (\%)}  & Average (\%) \\ 
\midrule
FT-TeCoA-1/255 \cite{mao2022understanding}          & 66.79  & 41.01  & 89.25  & 47.01  & 52.81  & 70.31  & 36.13  & 35.94  & 18.88  & 7.81   & 48.83   & 43.67   & 28.32   & 72.98   & 37.89   & 37.89   &46.99     \\
PMG-AFT-1/255(ours)    & 83.98  & 58.39  & 92.97  & 56.41  & 66.40  & 84.76  & 42.96  & 41.02  & 35.28  & 6.25   & 46.87   & 56.75   & 30.46   & 82.94   & 48.24   & 48.24   &\textbf{55.71}  \\ \hline
FT-TeCoA-2/255 \cite{mao2022understanding}       & 62.30  & 36.52 & 87.30  & 50.79 & 53.28 & 71.48 & 39.06 & 35.93 & 20.37 & 5.85 & 44.53 & 46.21 & 28.12 & 72.39 & 41.40  & 54.35 & 46.86  \\
PMG-AFT-2/255(ours)         & 78.12 & 54.29 & 91.01 & 56.94 & 65.15 & 85.54 & 41.01 & 37.89 & 31.96 & 4.29 & 35.15 & 54.60 & 29.49 & 79.29 & 46.09 & 54.68 & \textbf{52.84}   \\ \hline
FT-TeCoA-4/255  \cite{mao2022understanding}     & 62.50  & 38.86 & 89.45 & 57.33 & 63.59 & 80.46 & 42.96 & 37.50  & 29.36 & 3.51 & 40.82 & 53.94 & 28.12 & 76.95 & 42.07 & 49.88 & 49.83   \\
PMG-AFT-4/255(ours)         & 77.34 & 49.41 & 91.60  & 56.26 & 65.85 & 87.10  & 40.43 & 34.76 & 40.88 & 4.29 & 29.10  & 54.96 & 28.90  & 77.66 & 46.28 & 50.67 & \textbf{52.21}   \\
\bottomrule
\end{tabular}
\end{adjustbox}
\end{table*}
\begin{table*}[htbp]
\centering
\caption{Adversarial zero-shot robust accuracies under PGD-10 \cite{madry2017towards} attack. We fine-tune the model on TinyImageNet \cite{deng2009imagenet} by FT-TeCoA and our method with different loss function term coefficients and combinations. We evaluate on 16 datasets (columns), presenting the accuracy for each dataset as well as the average accuracy, with the best average result shown in bold. $\alpha$ and $\beta$ represent two hyper-parameters in the loss function $L=L_{robust}+\alpha L_{general}+\beta L_{clean}$.}
\label{tab:lossterm_detail_robust}
\begin{adjustbox}{width=\textwidth,keepaspectratio}
\begin{tabular}{lccccccccccccccccc}
\toprule
% & \multicolumn{16}{c}{\textbf{Datasets}} \\ % 合并中间的列，并在合并的列上添加标题 "Datasets"
% \cmidrule(lr){2-17} % 这个命令将会在从第二列到第十三列的上方画一条线，'lr'是为了减少线的长度
Method    & \scriptsize\rotatebox{90}{CIFAR10 (\%)} & \scriptsize\rotatebox{90}{CIFAR100 (\%)} & \scriptsize\rotatebox{90}{STL10 (\%)} & \scriptsize\rotatebox{90}{SUN397 (\%)} & \scriptsize\rotatebox{90}{Food101 (\%)} & \scriptsize\rotatebox{90}{Oxfordpet (\%)} & \scriptsize\rotatebox{90}{Flowers102 (\%)} & \scriptsize\rotatebox{90}{DTD (\%)}   & \scriptsize\rotatebox{90}{EuroSAT (\%)} & \scriptsize\rotatebox{90}{Fgvc\_Aircraft (\%)} & \scriptsize\rotatebox{90}{TinyImageNet (\%)} & \scriptsize\rotatebox{90}{ImageNet (\%)} & \scriptsize\rotatebox{90}{Caltech101 (\%)} & \scriptsize\rotatebox{90}{Caltech256 (\%)} & \scriptsize\rotatebox{90}{StanfordCars (\%)} & \scriptsize\rotatebox{90}{PCAM (\%)}  & Average (\%) \\ 
\midrule
FT-TeCoA \cite{mao2022understanding} ($\alpha=0,\beta=0$)          & 40.82 & 24.41 & 70.70  & 19.21 & 14.45 & 28.13 & 23.05 & 28.13 & 12.57 & 3.13 & 19.33 & 16.48 & 24.02 & 40.56 & 12.69 & 53.68 & 26.96    \\ \hline
PMG-AFT ($\alpha=1,\beta=0$) (ours)    & 55.46 & 29.29 & 73.24 & 21.48 & 10.70  & 27.73 & 18.55 & 31.64 & 25.58 & 0.78 & 6.64  & 14.37 & 17.38 & 48.69 & 14.84 & 58.89 & 28.44  \\ 
PMG-AFT ($\alpha=1,\beta=1$) (ours)       & 66.99 & 38.28 & 76.17 & 24.23 & 14.92 & 33.59 & 23.43 & 34.38 & 24.15 & 1.56 & 14.84 & 17.26 & 24.21 & 45.05 & 14.64 & 57.64 & \textbf{31.95}  \\
PMG-AFT ($\alpha=2,\beta=1$) (ours)         & 69.72 & 34.76 & 74.02 & 21.57 & 10.07 & 29.29 & 17.96 & 33.20  & 30.79 & 0.78 & 6.25  & 14.06 & 22.07 & 39.51 & 11.13 & 56.02 & 29.45   \\ 
PMG-AFT ($\alpha=1,\beta=2$) (ours)     & 65.43 & 38.67 & 77.93 & 25.03 & 15.31 & 36.32 & 24.21 & 35.93 & 23.50  & 0.78 & 16.99 & 17.69 & 24.21 & 46.74 & 14.25 & 57.36 & 31.52   \\
PMG-AFT ($\alpha=0.5,\beta=1$) (ours)         & 58.00    & 34.76 & 75.00    & 24.41 & 16.01 & 34.76 & 24.80  & 33.20  & 19.85 & 0.39 & 18.75 & 18.12 & 23.43 & 46.68 & 15.82 & 56.64 & 31.28   \\
PMG-AFT ($\alpha=1,\beta=0.5$) (ours)         & 64.84 & 36.91 & 75.58 & 23.29 & 13.67 & 30.85 & 22.65 & 33.98 & 24.87 & 1.17 & 11.13 & 16.32 & 22.46 & 44.66 & 13.67 & 57.81 & 30.86   \\
\bottomrule
\end{tabular}
\end{adjustbox}
\end{table*}
\begin{table*}[htbp]
\centering
\caption{Zero-shot clean accuracies. We fine-tune the model on TinyImageNet \cite{deng2009imagenet} by FT-TeCoA and our method with different loss function term coefficients and combinations. We evaluate on 16 datasets (columns), presenting the accuracy for each dataset as well as the average accuracy.
$\alpha$ and $\beta$ represent two hyper-parameters in the loss function $L=L_{robust}+\alpha L_{general}+\beta L_{clean}$.}
\label{tab:lossterm_detail_clean}
\begin{adjustbox}{width=\textwidth,keepaspectratio}
\begin{tabular}{lccccccccccccccccc}
\toprule
% & \multicolumn{16}{c}{\textbf{Datasets}} \\ % 合并中间的列，并在合并的列上添加标题 "Datasets"
% \cmidrule(lr){2-17} % 这个命令将会在从第二列到第十三列的上方画一条线，'lr'是为了减少线的长度
Method    & \scriptsize\rotatebox{90}{CIFAR10 (\%)} & \scriptsize\rotatebox{90}{CIFAR100 (\%)} & \scriptsize\rotatebox{90}{STL10 (\%)} & \scriptsize\rotatebox{90}{SUN397 (\%)} & \scriptsize\rotatebox{90}{Food101 (\%)} & \scriptsize\rotatebox{90}{Oxfordpet (\%)} & \scriptsize\rotatebox{90}{Flowers102 (\%)} & \scriptsize\rotatebox{90}{DTD (\%)}   & \scriptsize\rotatebox{90}{EuroSAT (\%)} & \scriptsize\rotatebox{90}{Fgvc\_Aircraft (\%)} & \scriptsize\rotatebox{90}{TinyImageNet (\%)} & \scriptsize\rotatebox{90}{ImageNet (\%)} & \scriptsize\rotatebox{90}{Caltech101 (\%)} & \scriptsize\rotatebox{90}{Caltech256 (\%)} & \scriptsize\rotatebox{90}{StanfordCars (\%)} & \scriptsize\rotatebox{90}{PCAM (\%)}  & Average (\%) \\ 
\midrule
FT-TeCoA \cite{mao2022understanding} ($\alpha=0,\beta=0$)          & 66.79 & 41.01 & 89.25 & 47.01 & 52.81 & 70.31 & 36.13 & 35.94 & 18.88 & 7.81 & 48.83 & 43.67 & 28.32 & 72.98 & 37.89 & 54.29 & 46.99     \\ \hline
PMG-AFT ($\alpha=1,\beta=0$) (ours)    & 86.52 & 65.43 & 95.89 & 57.81 & 71.95 & 83.20  & 44.14 & 42.18 & 46.41 & 9.37 & 61.13 & 60.62 & 24.21 & 80.07 & 43.94 & 59.61 & 58.28  \\ 
PMG-AFT ($\alpha=1,\beta=1$) (ours)       & 83.98 & 58.39 & 92.97 & 56.41 & 66.40  & 84.76 & 42.96 & 41.02 & 35.28 & 6.25 & 46.87 & 56.75 & 30.46 & 82.94 & 48.24 & 57.81 & 55.71  \\
PMG-AFT ($\alpha=2,\beta=1$) (ours)         & 87.30  & 59.76 & 94.33 & 57.58 & 71.09 & 84.37 & 43.75 & 40.62 & 51.56 & 7.42 & 35.54 & 58.94 & 31.44 & 83.46 & 51.95 & 56.19 & 57.20   \\ 
PMG-AFT ($\alpha=1,\beta=2$) (ours)     & 80.66 & 53.51 & 91.99 & 55.36 & 64.92 & 83.98 & 41.79 & 39.84 & 31.77 & 5.46 & 47.26 & 55.46 & 29.88 & 81.51 & 46.48 & 57.31 & 54.19   \\
PMG-AFT ($\alpha=0.5,\beta=1$) (ours)         & 77.93 & 51.56 & 91.40  & 53.92 & 63.51 & 82.81 & 42.18 & 38.67 & 28.97 & 6.25 & 50.39 & 54.10  & 29.29 & 80.40  & 45.89 & 56.75 & 53.37   \\
PMG-AFT ($\alpha=1,\beta=0.5$) (ours)         & 84.96 & 60.93 & 94.14 & 57.12 & 67.26 & 85.54 & 43.75 & 41.01 & 39.58 & 5.85 & 47.46 & 57.77 & 30.27 & 83.65 & 49.80  & 58.48 & 56.72   \\
\bottomrule
\end{tabular}
\end{adjustbox}
\end{table*}
\begin{table*}[htbp]
\centering
\caption{Adversarial zero-shot robust accuracies under PGD-10 \cite{madry2017towards} attack. We fine-tune the model on TinyImageNet \cite{deng2009imagenet} by our method under the selection of different feature layers and distance metric. We evaluate on 16 datasets (columns), presenting the accuracy for each dataset as well as the average accuracy, with the best results shown in bold.}
\label{tab:layer_robust}
\begin{adjustbox}{width=\textwidth,keepaspectratio}
\begin{tabular}{lccccccccccccccccc}
\toprule
% & \multicolumn{16}{c}{\textbf{Datasets}} \\ % 合并中间的列，并在合并的列上添加标题 "Datasets"
% \cmidrule(lr){2-17} % 这个命令将会在从第二列到第十三列的上方画一条线，'lr'是为了减少线的长度
Method    & \scriptsize\rotatebox{90}{CIFAR10 (\%)} & \scriptsize\rotatebox{90}{CIFAR100 (\%)} & \scriptsize\rotatebox{90}{STL10 (\%)} & \scriptsize\rotatebox{90}{SUN397 (\%)} & \scriptsize\rotatebox{90}{Food101 (\%)} & \scriptsize\rotatebox{90}{Oxfordpet (\%)} & \scriptsize\rotatebox{90}{Flowers102 (\%)} & \scriptsize\rotatebox{90}{DTD (\%)}   & \scriptsize\rotatebox{90}{EuroSAT (\%)} & \scriptsize\rotatebox{90}{Fgvc\_Aircraft (\%)} & \scriptsize\rotatebox{90}{TinyImageNet (\%)} & \scriptsize\rotatebox{90}{ImageNet (\%)} & \scriptsize\rotatebox{90}{Caltech101 (\%)} & \scriptsize\rotatebox{90}{Caltech256 (\%)} & \scriptsize\rotatebox{90}{StanfordCars (\%)} & \scriptsize\rotatebox{90}{PCAM (\%)}  & Average (\%) \\ 
\midrule
Output + KL          & \textbf{66.99} & \textbf{38.28} & \textbf{76.17} & \textbf{24.23} & \textbf{14.92}& \textbf{33.59}& \textbf{23.43}& \textbf{34.38} & \textbf{24.15}& \textbf{3.91} & 14.84& \textbf{17.26}& \textbf{24.02} & \textbf{45.05} & \textbf{14.64}& \textbf{57.64} &\textbf{31.95}     \\
Output + $L_2$    & 41.21 & 24.41 & 70.50  & 20.61 & 14.45 & 31.25 & 22.85 & 28.90  & 14.38 & 0.78 & 19.53 & 17.46 & 24.21 & 41.60  & 11.91 & 51.67 & 27.23  \\ 
Feature + $L_2$       & 40.62 & 21.09 & 70.50  & 11.61 & 11.71 & 20.70  & 8.33  & 8.59  & 10.44 & 0.39 & 28.12 & 14.33 & 17.96 & 37.95 & 9.57  & 54.50  & 22.90  \\
Feature + COS       & 53.32 & 28.12 & 67.77 & 13.33 & 10.23 & 29.68 & 14.58 & 12.50  & 10.01 & 1.17 & 10.15 & 14.14 & 16.40  & 43.88 & 13.47 & 53.84 & 24.53  \\
\bottomrule
\end{tabular}
\end{adjustbox}
\end{table*}
\begin{table*}[hbpt]
\centering
\caption{Zero-shot clean accuracies. We fine-tune the model on TinyImageNet \cite{deng2009imagenet} by our method under the selection of different feature layers and distance metric. We evaluate on 16 datasets (columns), presenting the accuracy for each dataset as well as the average accuracy, with the best average result shown in bold.}
\label{tab:layer_clean}
\begin{adjustbox}{width=\textwidth,keepaspectratio}
\begin{tabular}{lccccccccccccccccc}
\toprule
% & \multicolumn{16}{c}{\textbf{Datasets}} \\ % 合并中间的列，并在合并的列上添加标题 "Datasets"
% \cmidrule(lr){2-17} % 这个命令将会在从第二列到第十三列的上方画一条线，'lr'是为了减少线的长度
Method    & \scriptsize\rotatebox{90}{CIFAR10 (\%)} & \scriptsize\rotatebox{90}{CIFAR100 (\%)} & \scriptsize\rotatebox{90}{STL10 (\%)} & \scriptsize\rotatebox{90}{SUN397 (\%)} & \scriptsize\rotatebox{90}{Food101 (\%)} & \scriptsize\rotatebox{90}{Oxfordpet (\%)} & \scriptsize\rotatebox{90}{Flowers102 (\%)} & \scriptsize\rotatebox{90}{DTD (\%)}   & \scriptsize\rotatebox{90}{EuroSAT (\%)} & \scriptsize\rotatebox{90}{Fgvc\_Aircraft (\%)} & \scriptsize\rotatebox{90}{TinyImageNet (\%)} & \scriptsize\rotatebox{90}{ImageNet (\%)} & \scriptsize\rotatebox{90}{Caltech101 (\%)} & \scriptsize\rotatebox{90}{Caltech256 (\%)} & \scriptsize\rotatebox{90}{StanfordCars (\%)} & \scriptsize\rotatebox{90}{PCAM (\%)}  & Average (\%) \\ 
\midrule
Output + KL          & 83.98  & 58.39  & 92.97  & 56.41  & 66.40  & 84.76  & 42.96  & 41.02  & 35.28  & 6.25   & 46.87   & 56.75   & 30.46   & 82.94   & 48.24   & 48.24   &\textbf{55.71}     \\
Output + $L_2$    & 68.55 & 43.55 & 89.45 & 50.33 & 54.06 & 74.21 & 36.32 & 36.71 & 21.68 & 7.81  & 49.02 & 46.32 & 28.51 & 73.11 & 39.84 & 51.95 & 48.21  \\ 
Feature + $L_2$       & 59.18 & 31.83 & 86.52 & 33.73 & 31.40  & 42.18 & 21.09 & 17.96 & 15.90  & 17.57 & 56.05 & 33.59 & 25.19 & 59.44 & 22.26 & 59.31 & 38.32  \\
Feature + COS       & 80.66 & 48.63 & 93.55 & 55.52 & 67.10  & 68.35 & 39.58 & 35.93 & 36.29 & 16.79 & 42.38 & 54.18 & 24.41 & 81.90  & 49.21 & 53.24 & 52.98  \\
\bottomrule
\end{tabular}
\end{adjustbox}
\end{table*}

\section{Additional Experiments}
\label{sec:additionalExperiments}
\vspace{-1.5mm}

\hspace*{0.422cm}In Sec. \ref{exp_CIFAR100}, we supplement the main experiments on CIFAR100 \cite{krizhevsky2009learning}. 
Sec. \ref{streng_d} provides a detailed demonstration of the experiments regarding attack magnitude mentioned in the main manuscript. 
Furthermore, Sec. \ref{loss_d} and Sec. \ref{layer_d} are devoted to detailed ablation studies.
\vspace{-1.5mm}
\subsection{Experiments on CIFAR100}
\vspace{-1.5mm}
\label{exp_CIFAR100}
\hspace*{0.422cm}We also fine-tune the model on CIFAR100 \cite{krizhevsky2009learning} and evaluate it on all 16 datasets. 
Similarly, the evaluation except on the CIFAR-100 dataset is conducted in a zero-shot manner.
During training and evaluation, we use the PGD-10 \cite{madry2017towards} attack with a perturbation bound $\varepsilon = 1/255$. 
The robust accuracy results are shown in Tab. \ref{tab:cifar-robust}, and the clean accuracy results are displayed in Tab. \ref{tab:cifar-clean}.
We bold the best robust accuracy results for each dataset.

From Tab. \ref{tab:cifar-robust}, we can see that our method shows an average improvement in robust accuracy of 8.31\% compared with the original CLIP model. 
Compared with FT-TeCoA \cite{mao2022understanding}, the current state-of-the-art, our method shows an average improvement in robust accuracy of 4.71\%, and achieves improvement on the most of datasets except CIFAR100. 
However, the decrease observed on CIFAR-100 to some extent indicates that our method effectively mitigates the phenomenon of overfitting.
Moreover, Tab. \ref{tab:cifar-clean} demonstrates that the improvement in robust accuracy brought by the FT-TeCoA comes at the cost of a 4.03\% decrease in average clean accuracy compared with the original CLIP.
However, our method still outperforms FT-TeCoA in terms of clean accuracy, achieving a clean accuracy of 56.68\%.
For visual prompt, since it involves fewer parameters update than fine-tuning, both robust accuracy and clean accuracy are reduced across different methods. 
Nevertheless, our method consistently outperforms FT-TeCoA, further proving the effectiveness of our approach.

It is noteworthy that models fine-tuned on CIFAR100, as compared with those fine-tuned on TinyImageNet \cite{deng2009imagenet}, exhibit a decline in average robust accuracy for both our model and the model fine-tuned using FT-TeCoA. 
This also indicates that overfitting is more likely to occur on smaller-scale datasets.
Similar to the situation on TinyImageNet, our method results in an increase in computational cost, with each training epoch taking 124 seconds longer than FT-TeCoA. 
However, PMG-AFT achieves much better results in both average robust accuracy and clean accuracy than FT-TeCoA.
\vspace{-1.5mm}

\subsection{Detailed Results on Different Attack Strength}
\vspace{-1.5mm}
\label{streng_d}
\hspace*{0.422cm}We specifically present the experimental results on all datasets under different attack perturbation bounds. 
Consistent with the experimental setup in the main manuscript, we use the FT-TeCoA \cite{mao2022understanding} method and our PMG-AFT method on TinyImageNet to fine-tune models under perturbation bounds of $\varepsilon=1/255, 2/255$ and $4/255$, respectively. 
These models are tested under attacks of the same attack magnitude with training phrase. 

From Tab. \ref{tab:strength-robust} and \ref{tab:strength-clean}, it can be observed that with increasing perturbation, the robust accuracy of both methods decreases to varying degrees on each dataset. 
However, the degree of decrease is smaller for our method. 
Under different attack magnitudes, our method consistently achieves higher robust accuracy than FT-TeCoA \cite{mao2022understanding} on the majority of datasets, with average robust accuracies surpassing FT-TeCoA by 4.99\%, 4.70\%, and 4.86\% under perturbations of $1/255, 2/255$ and $4/255$, respectively.
Besides, as the size of adversarial perturbation continues to increase, the clean accuracy is almost unaffected, and our method consistently maintains performance superior to that of FT-TeCoA.
\vspace{-1.5mm}

\subsection{Ablation Study on Loss Function}
\vspace{-1.5mm}
\label{loss_d}
\hspace*{0.422cm}We provide a detailed demonstration of the contribution of each loss function term across each dataset.
As shown in Tab. \ref{tab:lossterm_detail_robust}, with the incorporation of our proposed $L_{general}$ loss (\ie, PMG-AFT ($\alpha=1,\beta=0$)), our method surpasses FT-TeCoA \cite{mao2022understanding} in robust accuracy on most datasets. 
However, there is a noticeable decline in the robust accuracy of our method on TinyImageNet \cite{deng2009imagenet}. 
With the introduction of another regularization loss, namely $L_{clean}$, the model's adversarial robust generalization is further enhanced, underscoring the significant potential of our approach.
For clean accuracy, as shown in Tab. \ref{tab:lossterm_detail_clean}, with the incorporation of our proposed loss, there is an obvious improvement compared with FT-TeCoA. 
The addition of $L_{general}$ alone achieves the best average accuracy on clean samples, and the results are optimal on most datasets.
This further confirms that our method effectively mitigates the phenomenon of overfitting.

We also adjust the coefficients preceding the two loss terms and find that with varying values of $\alpha$ and $\beta$, the robust and clean accuracies fluctuate within a certain range, yet consistently exhibit superior performance compared to FT-TeCoA. 
Ultimately, we discover that our method achieves the best average robust accuracy when $\alpha=1$ and $\beta=1$, and compared to other methods, it also attains the most optimal balance between robust and clean accuracies.
\vspace{-3mm}

\subsection{Ablation Study on Feature Layer and Distance Metric}
\vspace{-1.5mm}
\label{layer_d}
\hspace*{0.422cm}In Tab. \ref{tab:layer_robust} and Tab. \ref{tab:layer_clean}, we present in detail the robust and clean accuracies when applying KL divergence, $L_2$ distance, and cosine distance to the output layer and the penultimate feature layer across various datasets. 
Since the output layer represents a probability distribution, KL divergence distance can be directly applied, but this is not suitable for the feature layer. 
Moreover, cosine distance is generally not a common measure for probability vectors. 
Therefore, for the output layer, we only use KL distance and $L_2$ distance, while for the feature layer, we only employ $L_2$ distance and cosine distance.
The experimental results demonstrate that using KL divergence distance at the output layer achieves the best robust and clean accuracies, thereby proving the superiority of this choice.

We also observe that using the same $L_2$ distance, applying our loss function at the output layer results in better robust and clean accuracies than at the feature layer. 
Thus, the closer to the output layer, the more improvements are made from our method. 
Additionally, employing cosine distance measurement at the feature layer is a more suitable approach. 

Lastly, starting from the loss function, we simply derive the advantages of using KL distance measurement for $L_{general}$ at the output layer.
As shown in Equ, \eqref{KL_info}, $H(\cdot)$ represents entropy, $H(\cdot,\cdot)$ denotes cross-entropy, $I(\cdot,\cdot)$ denotes mutual information, $N$ is the size of a batch, $c$ is the number of categories, $Y$ represents the one-hot ground truth label, with a size of $N\times c$. 
$P_i$ represents the $i$-$th$ sample in a batch, and $j$ represents the $j$-$th$ element in the output probability tensor $P$.
For example, In \eqref{KL_info}, $P_{adv_{ij}}$ means The $j$-$th$ element of the output distribution obtained by inputting the $i$-$th$ adversarial example from a batch into the target model, $P_{ori_{ij}}$ means The $j$-$th$ element of the output distribution obtained by inputting the $i$-$th$ adversarial example from a batch into the pre-trained model.

We expand the formula in the loss function and simplify it using the knowledge of information theory.
Since the pre-trained model $F_{ori}(\cdot)$ is a fixed function, $H\left(P_{ori}\right)$ can be regarded as a constant.
Therefore, minimizing the loss function is equivalent to minimizing the cross entropy between adversarial examples and labels while maximizing the mutual information between the target model and the pre-trained model simultaneously, where the former is used to ensure robustness and the latter is used to ensure generalization transformation.
With the increase in mutual information between the target model and the pre-trained model, the target model is more likely to learn the generalized features of the pre-trained model.

\begin{figure}[htpb]
\begin{footnotesize}
\begin{equation}
\begin{aligned}
\label{KL_info}
& L_{robust }+L_{general } \\
& =-\frac{1}{N} \sum_{i=1}^N \sum_{j=1}^c Y_{ij} \log \left(P_{adv_{ij}}\right)+\frac{1}{N} \sum_{i=1}^N D_{KL}\left(P_{adv_i} \| P_{{ori_i}}\right) \\
& =-\frac{1}{N} \sum_{i=1}^N \sum_{j=1}^c Y_{ij} \log \left(P_{adv_{ij}}\right)+\frac{1}{N} \sum_{i=1}^N \sum_{j=1}^c P_{adv_{ij}} \log \left(\frac{P_{adv_{ij}}}{P_{ori_{ij}}}\right) \\
& =\frac{1}{N} \sum_{i=1}^N \sum_{j=1}^c[P_{adv_{ij}} \log \left(P_{adv_{ij}}\right)- P_{adv_{ij}} \log \left(P_{ori_{ij}}\right)-Y_{ij} \log \left(P_{adv_{ij}}\right)] \\
& =-H\left(P_{adv}\right)+H({P_{adv}, P_{ori}})+H\left(Y, P_{adv}\right) \\
& =-H\left(P_{adv}\right)+H\left(P_{adv}\right)+H\left(P_{ori }\right)-I(P_{adv}, P_{ori})+H\left(Y, P_{adv}\right) \\
& =H\left(P_{ori }\right)-I(P_{adv}, P_{ori})+H\left(Y, P_{adv}\right) \\
&
\end{aligned}
\end{equation}
\end{footnotesize}
\end{figure}

% \begin{equation}
% \begin{aligned}
% & L_{robust }+L_{general } \\
% & =-\frac{1}{N} \sum_{i=1}^N \sum_{j=1}^c Y_{ij} \log \left(P_{adv_{ij}}\right)+\frac{1}{N} \sum_{i=1}^N D_{KL}\left(P_{adv_i} \| P_{{ori_i}}\right) \\
% & =-\frac{1}{N} \sum_{i=1}^N \sum_{j=1}^c Y_{ij} \log \left(P_{adv_{ij}}\right)+\frac{1}{N} \sum_{i=1}^N \sum_{j=1}^c P_{adv_{ij}} \log \left(\frac{P_{adv_{ij}}}{P_{ori_{ij}}}\right) \\
% & =\frac{1}{N} \sum_{i=1}^N \sum_{j=1}^c\left[P_{adv_{ij}} \log \left(P_{adv_{ij}}\right)-P_{adv_{ij}} \log \left(P_{ori_{ij}}\right)-Y_{ij} \log \left(P_{adv_{ij}}\right)\right] \\
% & =-H\left(P_{adv}\right)+H({P_{adv}, P_{ori}})+H\left(Y, P_{adv}\right) \\
% & =-H\left(P_{adv}\right)+H\left(P_{adv}\right)+H\left(P_{ori }\right)-I(P_{adv}, P_{ori})+H\left(Y, P_{adv}\right) \\
% & =H\left(P_{ori }\right)-I(P_{adv}, P_{ori})+H\left(Y, P_{adv}\right) \\
% &
% \end{aligned}
% \end{equation}
